# Supplementary material for: Fast data inversion for high-dimensional Ornstein-Uhlenbeck processes from noisy measurements
Source: arXiv:2501.01324 ancillary file (2026-07-20)
Supplement: Supplementary file 1 [file supplement.pdf]

# SUPPLEMENTARY MATERIALS: Fast data inversion for high-dimensional dynamical systems from noisy measurements

Yizi Lin , Xubo Liu , Paul Segall , and Mengyang Gu

This file provides supplementary materials for "Fast data inversion for high-dimensional dynamical systems from noisy measurements". Section SM1 presents detailed proofs for Lemmas 2.1-2.3. SM2 reviews the Kalman filter and Rauch-Tung-Striebel smoother, which are essential for developing the proposed algorithm. Section SM3 derives the Exception-Maximization algorithm introduced in Section 2.2 of the main text. Section SM4 describes alternative methods, including dynamic mode decomposition, the network inversion filter (NIF), and modified NIF. Section SM5 provides additional numerical results of Experiments 2-5 to further demonstrate the FMOU's performance in uncertainty quantification. Finally, Section SM6 provides the details of the data preprocessing steps and model evaluation procedures for estimating the slip rate in Cascadia.

## SM1. Derivation for Lemmas 2.1-2.3.

### SM1.1. Proof of Lemma 2.1.

Before proving Lemma 2.1, we introduce three auxiliary facts.

1. Let $\mathbf{A}$ and $\mathbf{B}$ be $a \times a$ and $b \times b$ squared matrices, respectively. Then the Kronecker sum is defined as
$$\mathbf{A} \oplus \mathbf{B} = \mathbf{A} \otimes \mathbf{I}_a + \mathbf{I}_b \otimes \mathbf{B}.$$
where $\otimes$ denotes the Kronecker product, $\mathbf{I}_a$ and $\mathbf{I}_b$ are identity matrices with sizes $a \times a$ and $b \times b$, respectively.
2. Let $\mathbf{A}$ be a matrix,
$$e^{-(\mathbf{A}\oplus\mathbf{A})} = e^{(-\mathbf{A})\oplus(-\mathbf{A})} = e^{-\mathbf{A}} \otimes e^{-\mathbf{A}}.$$
3. For matrices $\mathbf{A}$, $\mathbf{B}$ and $\mathbf{C}$,
$$(\mathbf{C}^T \otimes \mathbf{A})\mathrm{vec}(\mathbf{B}) = \mathrm{vec}(\mathbf{ABC}).$$

*Proof of Lemma 2.1.* The discretization of the multivariate Ornstein-Uhlenbeck process described in Equation (5) can be written as [SM8]

$$\mathbf{m}(t+1) = e^{-\mathbf{U}_0\mathbf{D}\mathbf{U}_0^T}\mathbf{m}(t) + \boldsymbol{\varepsilon}(t+1), \tag{SM1.1}$$

where $\boldsymbol{\varepsilon}(t+1) \sim \mathcal{MN}(\mathbf{0}, \boldsymbol{\Sigma}_{\boldsymbol{\varepsilon}})$ with $\boldsymbol{\Sigma}_{\boldsymbol{\varepsilon}}$ satisfying $\big((\mathbf{U}_0\mathbf{D}\mathbf{U}_0^T)) \oplus (\mathbf{U}_0\mathbf{D}\mathbf{U}_0^T)\big)\,\mathrm{vec}(\boldsymbol{\Sigma}_{\boldsymbol{\varepsilon}}) = \Big(\mathbf{I} - e^{-((\mathbf{U}_0\mathbf{D}\mathbf{U}_0^T))\oplus(\mathbf{U}_0\mathbf{D}\mathbf{U}_0^T))}\Big)$ [illegible]

According to Equations (3)-(4), the evolution of the mean of the observation in our model can be expressed in a vector form:

$$\mathbf{m}(t+1) = \mathbf{C}\mathbf{m}(t) + \tilde{\mathbf{w}}(t+1), \tag{SM1.2}$$

where $\mathbf{C} = \mathbf{U}_0\mathrm{diag}(\rho_1, \dots, \rho_d)\mathbf{U}_0^T$ and $\tilde{\mathbf{w}}(t+1) = \mathbf{U}_0\mathrm{diag}(w_1(t+1), \dots, w_d(t+1)) \sim \mathcal{MN}(\mathbf{0}, \boldsymbol{\Sigma}_{\tilde{w}})$, with $w_l(t+1) \sim \mathcal{N}(0, \sigma_l^2)$ being the innovation of the $l$th latent factor and $\boldsymbol{\Sigma}_{\tilde{w}} = \mathbf{U}_0\mathrm{diag}(\sigma_1^2, \dots, \sigma_d^2)\mathbf{U}_0^T$.

We will show Equation (SM1.1) and Equation (SM1.2) are equivalent. First of all, as $\mathbf{D} = \text{diag}(-\log(\rho_1), \ldots, -\log(\rho_d))$, we have

$$e^{-\mathbf{U}_0\mathbf{D}\mathbf{U}_0^T} = \sum_{q=0}^{\infty} \frac{1}{q!} (-\mathbf{U}_0\mathbf{D}\mathbf{U}_0^T)^q = \mathbf{U}_0 \left( \sum_{q=0}^{\infty} \frac{(-\mathbf{D})^q}{q!} \right) \mathbf{U}_0^T = \mathbf{U}_0 \text{diag}(\rho_1, \ldots, \rho_d) \mathbf{U}_0^T = \mathbf{C},$$

where the the second equality holds as $\mathbf{U}_0^T\mathbf{U}_0 = \mathbf{I}_d$ and the third equality holds because $\mathbf{D}$ is a diagonal matrix and $\sum_{q=0}^{\infty} \frac{\log(\rho_l)^q}{q!} = e^{\log(\rho_l)} = \rho_l$ by the Taylor expansion.

Second, it suffices to show $\mathbf{\Sigma}_{\boldsymbol{\varepsilon}} = \mathbf{\Sigma}_{\tilde{w}}$ when $\tilde{\mathbf{D}} = \text{diag}\left( \sqrt{-2\frac{\sigma_1^2 \log(\rho_1)}{1-\rho_1^2}}, \ldots, \sqrt{-2\frac{\sigma_d^2 \log(\rho_d)}{1-\rho_d^2}} \right)$. This is equivalent to prove

(SM1.3)
$$\left((\mathbf{U}_0\mathbf{D}\mathbf{U}_0^T)) \oplus (\mathbf{U}_0\mathbf{D}\mathbf{U}_0^T)\right) \text{vec}\left(\mathbf{\Sigma}_{\tilde{w}}\right) = \left(\mathbf{I} - e^{-\left((\mathbf{U}_0\mathbf{D}\mathbf{U}_0^T))\oplus(\mathbf{U}_0\mathbf{D}\mathbf{U}_0^T)\right)}\right) \text{vec}(\mathbf{U}_0\tilde{\mathbf{D}}\tilde{\mathbf{D}}^T\mathbf{U}_0^T).$$

The left-hand side of Equation (SM1.3) can be expressed as:

$$\begin{aligned}
&\left((\mathbf{U}_0\mathbf{D}\mathbf{U}_0^T)) \oplus (\mathbf{U}_0\mathbf{D}\mathbf{U}_0^T)\right) \text{vec}\left(\mathbf{\Sigma}_{\tilde{w}}\right) \\
=& \left((\mathbf{U}_0\mathbf{D}\mathbf{U}_0^T) \otimes \mathbf{I}_k + \mathbf{I}_k \otimes (\mathbf{U}_0\mathbf{D}\mathbf{U}_0^T)\right) \text{vec}\left(\mathbf{U}_0\text{diag}(\sigma_1^2, \ldots, \sigma_d^2)\mathbf{U}_0^T\right) \\
=&\text{vec}\left( \mathbf{U}_0 \left( \mathbf{D}\text{diag}(\sigma_1^2, \ldots, \sigma_d^2) + \mathbf{D}\text{diag}(\sigma_1^2, \ldots, \sigma_d^2) \right) \mathbf{U}_0^T \right) \\
=&\text{vec}\left( \mathbf{U}_0\text{diag}(-2\log(\rho_1)\sigma_1^2, \ldots, -2\log(\rho_d)\sigma_d^2)\mathbf{U}_0^T \right),
\end{aligned}$$

where the first and second equalities use auxiliary Facts 1 and 3, respectively.

The right-hand side of Equation (SM1.3) can be expressed as:

$$\begin{aligned}
&\left(\mathbf{I} - e^{-\left((\mathbf{U}_0\mathbf{D}\mathbf{U}_0^T))\oplus(\mathbf{U}_0\mathbf{D}\mathbf{U}_0^T)\right)}\right) \text{vec}(\mathbf{U}_0\tilde{\mathbf{D}}\tilde{\mathbf{D}}^T\mathbf{U}_0^T) \\
=&\text{vec}(\mathbf{U}_0\tilde{\mathbf{D}}\tilde{\mathbf{D}}^T\mathbf{U}_0^T) - \left(e^{-\mathbf{U}_0\mathbf{D}\mathbf{U}_0^T} \otimes e^{-\mathbf{U}_0\mathbf{D}\mathbf{U}_0^T}\right) \text{vec}(\mathbf{U}_0\tilde{\mathbf{D}}\tilde{\mathbf{D}}^T\mathbf{U}_0^T) \\
=&\text{vec}(\mathbf{U}_0\tilde{\mathbf{D}}\tilde{\mathbf{D}}^T\mathbf{U}_0^T) - \text{vec}(\mathbf{C}\mathbf{U}_0\tilde{\mathbf{D}}\tilde{\mathbf{D}}^T\mathbf{U}_0^T\mathbf{C}) \\
=&\text{vec}\left( \mathbf{U}_0 \left( \tilde{\mathbf{D}}\tilde{\mathbf{D}}^T - \text{diag}(\rho_1, \ldots, \rho_d)\tilde{\mathbf{D}}\tilde{\mathbf{D}}^T\text{diag}(\rho_1, \ldots, \rho_d) \right) \mathbf{U}_0^T \right) \\
=&\text{vec}\left( \mathbf{U}_0\text{diag}(-2\log(\rho_1)\sigma_1^2, \ldots, -2\log(\rho_d)\sigma_d^2)\mathbf{U}_0^T \right), \quad \blacksquare
\end{aligned}$$

where the first equality utilizes auxiliary Fact 2, and the second equality is by Fact 3 and $\mathbf{C} = e^{-\mathbf{U}_0\mathbf{D}\mathbf{U}_0^T}$. Therefore, we've shown the left and right-hand sides in Equation (SM1.3) are the same. As a result, Equations (SM1.1) and (SM1.2) are equivalence.

## SM1.2. Proof of Lemma 2.2.

*Proof.* We first show that $\mathbb{V}[z_l(t)] = \rho_l^{2(t-1)}\tau_l^2 + \frac{1-\rho_l^{2(t-1)}}{1-\rho_l^2}\sigma_l^2$ for $t = 1, 2, \ldots, n$. We prove this by induction. For t=1, we have:

$$\mathbb{V}[z_l(1)] = \rho_l^0\tau_l^2 + \frac{1-\rho_l^2}{1-\rho_l^2}\sigma_l^2 = \tau_l^2.$$

Assume for $t > 1$, we have

$$\mathbb{V}[z_l(t)] = \rho_l^{2(t-1)}\tau_l^2 + \frac{1-\rho_l^{2(t-1)}}{1-\rho_l^2}\sigma_l^2. \tag{SM1.4}$$

Note for $t' > t$, Equation (SM1.4) leads to

$$\begin{aligned}
\mathrm{Cov}[z_l(t), z_l(t')] &= \mathrm{Cov}[z_l(t), \rho_l z_l(t'-1) + w_l(t')] \\
&= \rho_l \,\mathrm{Cov}[z_l(t), z_l(t'-1)] \\
&= \rho_l^{t'-t}\,\mathrm{Cov}[z_l(t), z_l(t)] \\
&= \rho_l^{t'-t}\left(\rho_l^{2(t-1)}\tau_l^2 + \frac{1-\rho_l^{2(t-1)}}{1-\rho_l^2}\sigma_l^2\right).
\end{aligned}$$

For any $t+1$, by Equation (4) and the law of total variance, the variance of $z_l(t+1)$ follows

$$\begin{aligned}
\mathbb{V}[z_l(t+1)] &= \mathbb{V}[\mathbb{E}(z_l(t+1)|z_l(t))] + \mathbb{E}[\mathbb{V}(z_l(t+1)|z_l(t))] \\
&= \rho_l^2\left(\rho_l^{2(t-1)}\tau_l^2 + \frac{1-\rho_l^{2(t-1)}}{1-\rho_l^2}\sigma_l^2\right) + \sigma_l^2 \\
&= \rho_l^{2t}\tau_l^2 + \frac{1-\rho_l^{2t}}{1-\rho_l^2}\sigma_l^2.
\end{aligned}$$

For $t' > t+1$,

$$\begin{aligned}
\mathrm{Cov}[z_l(t+1), z_l(t')] &= \mathrm{Cov}[z_l(t+1), \rho_l z_l(t'-1) + w_l(t')] \\
&= \rho_l\,\mathrm{Cov}[z_l(t+1), z_l(t'-1)] \\
&= \rho_l^{t'-t-1}\,\mathrm{Cov}[z_l(t+1), z_l(t+1)] \\
&= \rho_l^{t'-t-1}\left(\rho_l^{2t}\tau_l^2 + \frac{1-\rho_l^{2t}}{1-\rho_l^2}\sigma_l^2\right).
\end{aligned}$$

Thus, we've proved Equation (6).

When $\tau_l^2 = \frac{\sigma_l^2}{1-\rho_l^2}$, one can plug it into Equation (6) to obtain Equation (7). ∎

### SM1.3. Proof of Lemma 2.3 .

*Proof.* The tri-diagonal structure of $\mathbf{R}_l^{-1}$ can be directly proved by showing $\mathbf{R}_l\mathbf{R}_l^{-1} = \mathbf{I}_n$, where $\mathbf{I}_n$ is a $n \times n$ identity matrix.

To compute $|\mathbf{R}_l|$, note that the Cholesky decomposition to $\mathbf{R}_l$ such that $\mathbf{R}_l = \mathbf{L}_l\mathbf{L}_l^T$, where Cholesky factor follows

$$\mathbf{L}_l = \begin{pmatrix} 1 & 0 & 0 & \dots & 0 \\ \rho_l & \sqrt{1-\rho_l^2} & 0 & \dots & 0 \\ \rho_l^2 & \rho_l\sqrt{1-\rho_l^2} & \sqrt{1-\rho_l^2} & \cdots & 0 \\ \vdots & \vdots & \vdots & \ddots & \vdots \\ \rho_l^{n-1} & \rho_l^{n-2}\sqrt{1-\rho_l^2} & \rho_l^{n-3}\sqrt{1-\rho_l^3} & \dots & \sqrt{1-\rho_l^2} \end{pmatrix}.$$

Since $\mathbf{L}_l$ is a lower triangular matrix, $|\mathbf{L}_l| = |\mathbf{L}_l^T| = (1-\rho_l^2)^{(n-1)/2}$. Therefore, $|\mathbf{R}_l| = |\mathbf{L}_l||\mathbf{L}_l^T| = (1-\rho_l^2)^{(n-1)}$ and $|\mathbf{R}_l^{-1}| = \frac{1}{(1-\rho_l^2)^{n-1}}$. ■

## SM2. A review on Kalman filter and Rauch-Tung-Striebel smoother.

This section introduces the Kalman filter (KF) [SM6, SM7] and Rauch-Tung-Striebel (RTS) smoother [SM10], which will be applied to compute quantities the Expectation (E) step in our EM algorithm, speeding up the computation of Equation (11). Specifically, for each latent state $l$, the conditional mean $\hat{\mathbf{z}}_l$, conditional variance $\mathbb{V}[z_l(t) \mid \mathbf{Y}, \hat{\mathbf{\Theta}}]$ for $t = 1, \dots, n$, and conditional covariance $\mathrm{Cov}[z_l(t), z_l(t+1) \mid \mathbf{Y}, \hat{\mathbf{\Theta}}]$ for $t = 1, \dots, n-1$ can be obtained by KF and RTS smoother with computational order $\mathcal{O}(n)$. Inheriting from our assumptions about the data, we consider the following one-dimensional dynamic linear model for each latent factor and treat the projected data $\tilde{\mathbf{y}}_l$ as observation. The subscript $l$ is dropped for simplicity.

$$\tilde{y}(t) = z(t) + \epsilon(t), \quad \epsilon(t) \sim \mathcal{N}(0, \sigma_0^2),$$
$$z(t) = \rho z(t-1) + w(t), \quad w(t) \sim \mathcal{N}(0, \sigma^2),$$

for $t = 2, \dots, n$ and $z(1) \sim \mathcal{N}(m(1), C(1))$.

The KF and RTS Smoother are commonly referred to as the forward filtering and backward smoothing (FFBS) algorithm (see e.g. [SM13, SM9, SM4]). The KF and RTS Smoother are not contributions of this work. Here we summarize these results and give the proof of results for completeness as these will be used to derive closed-form expressions of the quantities in the EM algorithm.

### SM2.1. Kalman filter.

Denote $\tilde{\mathbf{y}}_{1:t} = \left(\tilde{y}(1), \dots, \tilde{y}(t)\right)^T$ and

$$z(t-1) \mid \tilde{\mathbf{y}}_{1:t-1} \sim \mathcal{N}\left(m(t-1), C(t-1)\right).$$

By Kalman filter, one can get the conditional distribution of $z(t) \mid \tilde{\mathbf{y}}_{1:t}$, for $t = 2, \dots, n$. We start from the one-step-ahead prediction of $z(t)$ given $\tilde{\mathbf{y}}_{1:t-1}$:

$$z(t) \mid \tilde{\mathbf{y}}_{1:t-1} \sim \mathcal{N}(\alpha(t), R(t)),$$

where

$$\alpha(t) = \rho m(t-1),$$
$$R(t) = \rho^2 C(t-1) + \sigma^2.$$

The one-step-ahead prediction of $\tilde{y}(t)$ given $\tilde{\mathbf{y}}_{1:t-1}$ is

$$\tilde{y}(t) \mid \tilde{\mathbf{y}}_{1:t-1} \sim \mathcal{N}(f(t), Q(t)),$$

where

$$f(t) = \alpha(t),$$
$$Q(t) = R(t) + \sigma_0^2.$$

The filtering distribution of $z(t)$ given $\tilde{\mathbf{y}}_{1:t}$ is

$$z(t) \mid \tilde{\mathbf{y}}_{1:t} \sim \mathcal{N}(m(t), C(t)),$$

where

$$m(t) = \alpha(t) + R(t)Q(t)^{-1}(\tilde{y}(t) - f(t)),$$
$$C(t) = R(t) - R(t)Q(t)^{-1}R(t).$$

*Proof.* For the one-step-ahead predictive distribution of $z(t)$ given $\tilde{\mathbf{y}}_{1:t-1}$,

$$\alpha_t = \mathbb{E}[z(t) \mid \tilde{\mathbf{y}}_{1:t-1}] = \mathbb{E}[\mathbb{E}[z(t) \mid z(t-1), \tilde{\mathbf{y}}_{1:t-1}]] = \mathbb{E}[\rho z(t-1) \mid \tilde{\mathbf{y}}_{1:t-1}] = \rho m(t-1),$$
$$\begin{aligned} R(t) &= \mathbb{V}[z(t) \mid \tilde{\mathbf{y}}_{1:t-1}] \\ &= \mathbb{V}[\mathbb{E}[z(t) \mid z(t-1), \tilde{\mathbf{y}}_{1:t-1}]] + \mathbb{E}[\mathbb{V}[z(t) \mid z(t-1), \tilde{\mathbf{y}}_{1:t-1}]] \\ &= \mathbb{V}[\rho z(t-1) \mid \tilde{\mathbf{y}}_{1:t-1}] + \mathbb{E}[\sigma^2 \mid \tilde{\mathbf{y}}_{1:t-1}] \\ &= \rho^2 C(t-1) + \sigma^2. \end{aligned}$$

For the one-step-ahead predictive distribution of $\tilde{y}(t)$ given $\tilde{\mathbf{y}}_{1:t-1}$,

$$\begin{aligned} f(t) &= \mathbb{E}[\tilde{y}(t) \mid \tilde{\mathbf{y}}_{1:t-1}] = \mathbb{E}[\mathbb{E}[\tilde{y}(t) \mid z(t), \tilde{\mathbf{y}}_{1:t-1}]] = \mathbb{E}[z(t) \mid \tilde{\mathbf{y}}_{1:t-1}] = \alpha(t) \\ Q(t) &= \mathbb{V}[\tilde{y}(t) \mid \tilde{\mathbf{y}}_{1:t-1}] \\ &= \mathbb{V}[\mathbb{E}[\tilde{y}(t) \mid z(t), \tilde{\mathbf{y}}_{1:t-1}]] + \mathbb{E}[\mathbb{V}[\tilde{y}(t) \mid z(t), \tilde{\mathbf{y}}_{1:t-1}]] \\ &= \mathbb{V}[z(t) \mid \tilde{\mathbf{y}}_{1:t-1}] + \mathbb{E}[\sigma_0^2] \\ &= R(t) + \sigma_0^2. \end{aligned}$$

For the filtering distribution of $z(t)$ given $\tilde{\mathbf{y}}_{1:t}$, we start from the conditional joint distribution of $(\tilde{y}(t), z(t))^T$ given $\tilde{\mathbf{y}}_{1:t-1}$:

$$\begin{pmatrix} \tilde{y}(t) \\ z(t) \end{pmatrix} \mid \tilde{\mathbf{y}}_{1:t-1} \sim \mathcal{MN}\left( \begin{pmatrix} f(t) \\ \alpha(t) \end{pmatrix}, \begin{pmatrix} Q(t) & R(t) \\ R(t) & R(t) \end{pmatrix} \right).$$

Thus, by the conditional distributions of normal distribution, we have

$$\begin{aligned} m(t) &= \mathbb{E}[z(t) \mid \tilde{\mathbf{y}}_{1:t}] = \mathbb{E}[z(t) \mid \tilde{\mathbf{y}}_{1:t}] = \alpha(t) + R(t)Q^{-1}(t)(\tilde{y}(t) - f(t)), \\ C(t) &= \mathbb{V}[z(t) \mid \tilde{\mathbf{y}}_{1:t}] = \mathbb{V}[z(t) \mid \tilde{\mathbf{y}}_{1:t}] = R(t) - R(t)Q^{-1}(t)R(t). \end{aligned}$$

∎

**SM2.2. Rauch-Tung-Striebel smoother.** From the Kalman filter, we only get the distribution of $(z(t) \mid \tilde{\mathbf{y}}_{1:t})$ but not $(z(t) \mid \tilde{\mathbf{y}}_{1:n})$, which is required for Equation (11), for any $t < n$. This can be achieved by a backward smoothing step. Suppose the posterior distribution of $z(t+1)$ conditional on full data $\tilde{\mathbf{y}}_{1:n}$ is $(z(t+1) \mid \tilde{\mathbf{y}}_{1:n}) \sim \mathcal{N}(s(t+1), S(t+1))$, then the conditional distribution $(z(t) \mid \tilde{\mathbf{y}}_{1:n})$ is:

$$z(t) \mid \tilde{\mathbf{y}}_{1:n} \sim \mathcal{N}(s(t), S(t)),$$

where

$$\begin{aligned} s(t) &= m(t) + \rho C(t) R^{-1}(t+1)(s(t+1) - a(t+1)), \\ S(t) &= C(t) - \rho^2 C(t) R^{-1}(t+1)(R(t+1) - S(t+1)) R^{-1}(t+1) C(t). \end{aligned}$$

Further, the covariance between $z(t)$ and $z(t+1)$ conditional on $\tilde{\mathbf{y}}_{1:n}$ for $t = 1, 2, \ldots, n-1$ is

$$\tilde{S}(t) = \mathrm{Cov}[z(t), z(t+1) \mid \tilde{\mathbf{y}}_{1:n}] = \rho C(t) R^{-1}(t+1) S(t+1).$$

*Proof.* We first show the derivation of $s(t)$ and $S(t)$. Notice that $p\,(z(t) \mid z(t+1), \tilde{\mathbf{y}}_{1:n}) = p\,(z(t) \mid z(t+1), \tilde{\mathbf{y}}_{1:t})$ and $p\,(z(t+1) \mid z(t), \tilde{\mathbf{y}}_{1:t}) = p\,(z(t+1) \mid z(t))$. The conditional distribution of $(z(t+1), z(t))^T$ given $\tilde{\mathbf{y}}_{1:t}$ is:

$$\begin{pmatrix} z(t+1) \\ z(t) \end{pmatrix} \mid \tilde{\mathbf{y}}_{1:t} \sim \mathcal{MN}\left( \begin{pmatrix} \alpha(t+1) \\ m(t) \end{pmatrix}, \begin{pmatrix} R(t+1) & \rho C(t) \\ \rho C(t) & C(t) \end{pmatrix} \right).$$

Therefore,

$$\begin{aligned} \mathbb{E}[z(t) \mid z(t+1), \tilde{\mathbf{y}}_{1:t}] &= m(t) + \rho C(t) R^{-1}(t+1)(z(t+1) - \alpha(t+1)) \\ \mathbb{V}[z(t) \mid z(t+1), \tilde{\mathbf{y}}_{1:t}] &= C(t) - \rho^2 C(t) R^{-1}(t+1) C(t), \end{aligned}$$

from which one has

$$\begin{aligned} s(t) &= \mathbb{E}[z(t) \mid \tilde{\mathbf{y}}_{1:n}] \\ &= \mathbb{E}[\mathbb{E}[z(t) \mid z(t+1), \tilde{\mathbf{y}}_{1:n}]] \\ &= \mathbb{E}[m(t) + \rho C(t) R^{-1}(t+1)(z(t+1) - \alpha(t+1)) \mid \tilde{\mathbf{y}}_{1:n}] \\ &= m(t) + \rho C(t) R^{-1}(t+1)(s(t+1) - \alpha(t+1)), \end{aligned}$$

and

$$\begin{aligned} S(t) &= \mathbb{V}[z(t) \mid \tilde{\mathbf{y}}_{1:n}] \\ &= \mathbb{V}[\mathbb{E}[z(t) \mid z(t+1), \tilde{\mathbf{y}}_{1:n}]] + \mathbb{E}[\mathbb{V}[z(t) \mid z(t+1), \tilde{\mathbf{y}}_{1:n}]] \\ &= \rho^2 C(t) R^{-1}(t+1) S(t+1) R(t+1) C(t) + (C(t) - \rho^2 C(t) R^{-1}(t+1) C(t)) \\ &= C(t) - \rho^2 C(t) R^{-1}(t+1)(R(t+1) - S(t+1)) R^{-1}(t+1) C(t). \end{aligned}$$

For the covariance between $z(t)$ and $z(t+1)$ conditional on $\tilde{\mathbf{y}}_{1:n}$,

$$\begin{aligned}
&\tilde{S}(t) = \mathrm{Cov}[z(t), z(t+1) \mid \tilde{\mathbf{y}}_{1:n}] \\
=&\mathbb{E}[\mathrm{Cov}[z(t), z(t+1) \mid z(t+1), \tilde{\mathbf{y}}_{1:n}]] \\
&+ \mathrm{Cov}[\mathbb{E}[z(t)|z(t+1), \tilde{\mathbf{y}}_{1:n}], \mathbb{E}[z(t+1)|z(t+1), \tilde{\mathbf{y}}_{1:n}]] \\
=&0 + \mathrm{Cov}[m(t) + \rho C(t)R^{-1}(t+1)(z(t+1) - \alpha(t+1)), z(t+1) \mid \tilde{\mathbf{y}}_{1:n}] \\
=&\rho C(t)R^{-1}(t+1)S(t+1).
\end{aligned}$$

■

*Remark* SM2.1. Consider a dynamic linear model with the $l$th row of the projected data $\tilde{\mathbf{Y}}$ being the observations and the $l$th latent process being the state vector:

$$\begin{aligned}
\tilde{y}_l(t) &= z_l(t) + \epsilon(t), \quad \epsilon(t) \sim \mathcal{N}(0, \sigma_0^2), \\
z_l(t) &= \rho_l z_l(t-1) + w_l(t), \quad w_l(t) \sim \mathcal{N}(0, \sigma_l^2).
\end{aligned}$$

By applying KF and RTS smoother, one can compute the posterior mean and variance of $z_l(t)$, denoted as $s_l(t)$ and $S_l(t)$, respectively, as well as the posterior covariance between $z_l(t)$ and $z_l(t+1)$, denoted as $\tilde{S}_l(t)$.

Therefore, the posterior mean of the $l$th latent factor can be obtained by

$$\hat{\mathbf{z}}_l = \mathbb{E}[\mathbf{z}_l \mid \mathbf{Y}, \hat{\mathbf{\Theta}}] = [s_l(1), \ldots, s_l(n)]^T.$$

The diagonal terms of the posterior covariance matrix $\hat{\sigma}_0^2\hat{\mathbf{\Sigma}}_l(\hat{\mathbf{\Sigma}}_l+\sigma_0^2\mathbf{I}_n)^{-1}$ in Equation (2.10),which are the posterior variance of $\mathbf{z}_l$, can be obtained by

$$\mathbb{V}[\mathbf{z}_l \mid \mathbf{Y}, \hat{\mathbf{\Theta}}] = [S_l(1), \ldots, S_l(n)]^T.$$

The primary off-diagonal terms of the posterior covariance matrix $\hat{\sigma}_0^2\hat{\mathbf{\Sigma}}_l(\hat{\mathbf{\Sigma}}_l + \sigma_0^2\mathbf{I}_n)^{-1}$, which are the posterior covariance between $z_l(t)$ and $z_l(t+1)$ for $t = 1, \ldots, n-1$, are $[\tilde{S}_l(1), \ldots, \tilde{S}_l(n-1)]^T$. The total computational order for calculating the posterior mean, diagonal and primary off-diagonal elements of the posterior covariance matrix of $d$ latent factors is $\mathcal{O}(dn)$. Lemma 2.4 gives the details on utilizing these quantities.

## SM3. Derivation for Section 2.2 .

We are ready to show the derivation of the Expectation-Maximization (EM) algorithm. We start from a general scenario where the parameters $\mathbf{\Theta} = (\mathbf{U}_0, \sigma_0^2, \boldsymbol{\sigma}, \boldsymbol{\rho})$ are unknown. Then we modify our algorithm to special applications where $\mathbf{U}_0$ and $\sigma_0^2$ are given.

**SM3.1. Proof of Equation (9).** The EM algorithm begins with the natural logarithm of the joint likelihood of the observations $\mathbf{Y}$ and the latent factors $\mathbf{Z} = [\mathbf{z}_1, \dots, \mathbf{z}_d]^T$.

$$\begin{aligned}\ell(\mathbf{\Theta}) &= \log\left(p(\mathbf{Y}, \mathbf{Z} \mid \mathbf{\Theta})\right)\\ &= \log\left(p(\mathbf{Y} \mid \mathbf{Z}, \mathbf{\Theta})\right) + \log\left(p(\mathbf{Z} \mid \mathbf{\Theta})\right)\\ &= C - \frac{nk}{2}\log(\sigma_0^2) - \sum_{t=1}^{n} \frac{(\mathbf{y}(t) - \mathbf{U}_0\mathbf{z}(t))^T(\mathbf{y}(t) - \mathbf{U}_0\mathbf{z}(t))}{2\sigma_0^2}\\ &\quad - \sum_{l=1}^{d}\left(\frac{\log|\mathbf{\Sigma}_l| + \mathbf{z}_l^T\mathbf{\Sigma}_l^{-1}\mathbf{z}_l}{2}\right)\\ &= C - \frac{nk}{2}\log(\sigma_0^2) - \frac{\mathrm{tr}(\mathbf{Y}^T\mathbf{Y} - 2\mathbf{Y}^T\mathbf{U}_0\mathbf{Z})}{2\sigma_0^2} - \sum_{l=1}^{d}\left(\frac{\mathbf{z}_l^T\mathbf{z}_l}{2\sigma_0^2} + \frac{\log|\mathbf{\Sigma}_l| + \mathbf{z}_l^T\mathbf{\Sigma}_l^{-1}\mathbf{z}_l}{2}\right),\end{aligned}$$

where $C = -\frac{(nk+nd)}{2}\log(2\pi)$ is a constant, $\tilde{\mathbf{Y}} = \mathbf{U}_0^T\mathbf{Y} = [\tilde{\mathbf{y}}_1, \cdots, \tilde{\mathbf{y}}_d]^T$ is the $d \times n$ projected observation matrix.

**SM3.2. Proof of Equation (11).** In the Expectation (E) step we calculate the expectation of Equation (9) with respect to the distribution of latent factor $\mathbf{Z}$, conditional on data $\mathbf{Y}$ and the current estimated parameters $\hat{\mathbf{\Theta}} = (\hat{\mathbf{U}}_0, \hat{\sigma}_0^2, \hat{\boldsymbol{\rho}}, \hat{\boldsymbol{\sigma}}^2)$. Making use of the expectation of quadratic forms, we obtain the expectation of $\ell(\mathbf{\Theta})$ as follows:

$$\begin{aligned}\bar{\ell}(\mathbf{\Theta}) :&= \mathbb{E}_{\mathbf{Z}|\mathbf{Y},\hat{\mathbf{\Theta}}}[\ell(\mathbf{\Theta})]\\ &= C - \frac{nk}{2}\log(\sigma_0^2) - \frac{\mathrm{tr}(\mathbf{Y}^T\mathbf{Y})}{2\sigma_0^2} + \frac{\mathbb{E}_{\mathbf{Z}|\mathbf{Y},\hat{\mathbf{\Theta}}}[\mathrm{tr}(\mathbf{Y}^T\mathbf{U}_0\mathbf{Z})]}{\sigma_0^2} - \sum_{l=1}^{d}\frac{\mathbb{E}_{\mathbf{Z}|\mathbf{Y},\hat{\mathbf{\Theta}}}[\mathbf{z}_l^T\mathbf{z}_l]}{2\sigma_0^2}\\ &\quad - \sum_{l=1}^{d}\frac{\log|\mathbf{\Sigma}_l| + \mathbb{E}_{\mathbf{Z}|\mathbf{Y},\hat{\mathbf{\Theta}}}[\mathbf{z}_l^T\mathbf{\Sigma}_l^{-1}\mathbf{z}_l]}{2}\\ &= C - \frac{nk}{2}\log(\sigma_0^2) - \frac{\mathrm{tr}(\mathbf{Y}^T\mathbf{Y})}{2\sigma_0^2} + \frac{\mathrm{tr}(\mathbf{Y}^T\mathbf{U}_0\hat{\mathbf{Z}})}{\sigma_0^2} - \sum_{l=1}^{d}\frac{\hat{\mathbf{z}}_l^T\hat{\mathbf{z}}_l + \mathrm{tr}[\hat{\sigma}_0^2\hat{\mathbf{\Sigma}}_l(\hat{\mathbf{\Sigma}}_l + \hat{\sigma}_0^2\mathbf{I}_n)^{-1}]}{2\sigma_0^2}\\ &\quad - \sum_{l=1}^{d}\frac{\log|\mathbf{\Sigma}_l| + \hat{\mathbf{z}}_l^T\mathbf{\Sigma}_l^{-1}\hat{\mathbf{z}}_l + \mathrm{tr}[\hat{\sigma}_0^2\mathbf{\Sigma}_l^{-1}\hat{\mathbf{\Sigma}}_l(\hat{\mathbf{\Sigma}}_l + \hat{\sigma}_0^2\mathbf{I}_n)^{-1}]}{2},\end{aligned}$$

where $\hat{\mathbf{z}}_l = \mathbb{E}[\mathbf{z}_l \mid \mathbf{Y}, \hat{\mathbf{\Theta}}]$, $\hat{\mathbf{Z}} = [\hat{\mathbf{z}}_1, \dots, \hat{\mathbf{z}}_d]^T$.

**SM3.3. Proof of Lemma 2.4.**

*Proof.* First, for $l = 1, 2, \dots, n$, by definition of KF and RTS smoother, one has

$$\hat{\mathbf{Z}} = [\hat{\mathbf{z}}_1, \dots, \hat{\mathbf{z}}_d]^T, \quad \text{with } \hat{\mathbf{z}}_l = [s_l(1), s_l(2), \dots, s_l(n)]^T,$$

$$\mathrm{tr}[\hat{\sigma}_0^2\hat{\mathbf{\Sigma}}_l(\hat{\mathbf{\Sigma}}_l + \hat{\sigma}_0^2\mathbf{I}_n)^{-1}] = \sum_{t=1}^{n}\mathbb{V}[\mathbf{z}_l(t) \mid \mathbf{Y}, \hat{\mathbf{\Theta}}] = \sum_{t=1}^{n} S_l(t),$$

where $s_l(t) = \mathbb{E}[z_l(t) \mid \mathbf{Y}, \hat{\boldsymbol{\Theta}}]$ and $S_l(t) = \mathbb{V}[z_l(t) \mid \mathbf{Y}, \hat{\boldsymbol{\Theta}}]$ for $t = 1, \ldots, n$ can be obtained by applying KF and RTS smoother to the $l$-th latent process with complexity $\mathcal{O}(n)$.

Second, by utilizing the tri-diagonal structure of $\boldsymbol{\Sigma}_l^{-1}$, as shown in Lemma 2.3, one has

$$\begin{aligned}\hat{\mathbf{z}}_l^T \boldsymbol{\Sigma}_l^{-1} \hat{\mathbf{z}}_l &= \frac{1}{\sigma_l^2} \begin{pmatrix} s_l(1) \\ s_l(2) \\ \vdots \\ \vdots \\ s_l(n) \end{pmatrix}^T \begin{pmatrix} 1 & -\rho_l & 0 & 0 & \cdots \\ -\rho_l & 1+\rho_l^2 & -\rho_l & 0 & \cdots \\ 0 & -\rho_l & 1+\rho_l^2 & \ddots & \\ \vdots & \vdots & \ddots & \ddots & -\rho_l \\ 0 & 0 & \cdots & -\rho_l & 1 \end{pmatrix} \begin{pmatrix} s_l(1) \\ s_l(2) \\ \vdots \\ \vdots \\ s_l(n) \end{pmatrix} \\ &= \frac{1}{\sigma_l^2} \left( (1-\rho_l^2) s_l(1) + \sum_{t=2}^{n} (s_l(t) - \rho_l s_l(t-1))^2 \right).\end{aligned}$$

$$\begin{aligned}&\operatorname{tr}[\hat{\sigma}_0^2 \boldsymbol{\Sigma}_l^{-1} \hat{\boldsymbol{\Sigma}}_l (\hat{\boldsymbol{\Sigma}}_l + \hat{\sigma}_0^2 \mathbf{I}_n)^{-1}] \\ &= \operatorname{tr}\left( \begin{pmatrix} \frac{1}{\sigma_l^2} & -\frac{\rho_l}{\sigma_l^2} & 0 & 0 & \cdots \\ -\frac{\rho_l}{\sigma_l^2} & \frac{1+\rho_l^2}{\sigma_l^2} & \frac{-\rho_l}{\sigma_l^2} & 0 & \cdots \\ 0 & -\frac{\rho_l}{\sigma_l^2} & \frac{1+\rho_l^2}{\sigma_l^2} & \ddots & \cdots \\ \vdots & \vdots & \ddots & \ddots & -\frac{\rho_l}{\sigma_l^2} \\ 0 & 0 & \cdots & -\frac{\rho_l}{\sigma_l^2} & \frac{1}{\sigma_l^2} \end{pmatrix} \begin{pmatrix} S_l(1) & \tilde{S}_l(1) & \cdot & \cdot & \cdots & \cdot \\ \tilde{S}_l(1) & S_l(2) & \tilde{S}_l(2) & \cdot & \cdots & \cdot \\ \cdot & \tilde{S}_l(2) & S_l(3) & \tilde{S}_l(3) & \cdots & \cdot \\ & & \ddots & \ddots & \ddots & \\ \vdots & \vdots & \vdots & \ddots & \ddots & \tilde{S}_l(n-1) \\ \cdot & \cdot & \cdot & \cdot & \tilde{S}_l(n-1) & S_l(n) \end{pmatrix} \right) \\ &= \frac{1}{\sigma_l^2} \left( \sum_{t=1}^{n} S_l(t) + \rho_l^2 \sum_{t=2}^{n-1} S_l(t) - 2\rho_l \sum_{t=1}^{n-1} \tilde{S}_l(t) \right),\end{aligned}$$

where $\tilde{S}_l(t) = \operatorname{Cov}[z_l(t), z_l(t+1) \mid \mathbf{Y}, \hat{\boldsymbol{\Theta}}]$ for $t = 1, \ldots, n-1$ can be obtained by applying KF and RTS smoother to the $l$-th latent process with computational complexity $\mathcal{O}(n)$.

Therefore, Equation (11) can be written as

$$\begin{aligned}&\bar{\ell}(\boldsymbol{\Theta}) \\ &= C - \frac{nk}{2} \log(\sigma_0^2) + \frac{\operatorname{tr}(\mathbf{Y}^T \mathbf{U}_0 \hat{\mathbf{Z}})}{\sigma_0^2} - \sum_{l=1}^{d} \left\{ \frac{1}{2} \log \frac{\sigma_l^{2n}}{1-\rho_l^2} + \frac{\sum_{t=1}^{n} (s_l^2(t) + S_l(t))}{2\sigma_0^2} \right\} - \frac{\operatorname{tr}(\mathbf{Y}^T \mathbf{Y})}{2\sigma_0^2} \\ &\quad - \sum_{l=1}^{d} \frac{(1-\rho_l^2) s_l(1) + \sum_{t=2}^{n} (s_l(t) - \rho_l s_l(t-1))^2 + \sum_{t=1}^{n} S_l(t) + \rho_l^2 \sum_{t=2}^{n-1} S_l(t) - 2\rho_l \sum_{t=1}^{n-1} \tilde{S}_l(t)}{2\sigma_l^2}. \blacksquare\end{aligned}$$

## SM3.4. Proof of Theorem 2.5.

*Proof.* By leveraging Equation (11) and Lemma 2.4 , estimating $\mathbf{U}_0$ is equivalent to maximizing $\operatorname{tr}(\hat{\mathbf{Z}} \mathbf{Y}^T \mathbf{U}_0)$ with the constrain $\mathbf{U}_0^T \mathbf{U}_0 = \mathbf{I}_d$. This is a linear optimization on Stiefel

manifold (see Proposition 2.5 in [SM14]). Denote the SVD of $\mathbf{Z}\mathbf{Y}^T = \tilde{\mathbf{U}}\tilde{\mathbf{D}}\tilde{\mathbf{V}}^T$. The objective function is then

$$\text{tr}\left[\hat{\mathbf{Z}}\mathbf{Y}^T\mathbf{U}_0\right] = \text{tr}\left[\tilde{\mathbf{U}}\tilde{\mathbf{D}}\tilde{\mathbf{V}}^T\mathbf{U}_0\right] = \text{tr}\left[\tilde{\mathbf{D}}\tilde{\mathbf{V}}^T\mathbf{U}_0\tilde{\mathbf{U}}\right]. \tag{SM3.1}$$

Denote $\tilde{\mathbf{V}}^T\mathbf{U}_0\tilde{\mathbf{U}} := [\mathbf{m}_1, ..., \mathbf{m}_d] := \mathbf{M}$ a $d \times d$ orthogonal matrix. As $||\mathbf{m}_l|| = 1$ for $l = 1, \ldots, d$, the diagonal terms of $\mathbf{M}$ is not larger than one. As the diagonal term in $\tilde{\mathbf{D}}$ is nonnegative, the maximum values are obtained when diagonal values of $\mathbf{M}$ are 1 or equivalently when

$$\tilde{\mathbf{V}}^T\hat{\mathbf{U}}_0^{\text{new}}\tilde{\mathbf{U}} = \mathbf{I}_d,$$

from which Equation (16) is proved.

After obtaining $\mathbf{U}_0^{\text{new}}$, compute $\tilde{\mathbf{Y}} = (\hat{\mathbf{U}}_\mathbf{0}^{\text{new}})^T\mathbf{Y}$ and denote $\tilde{\mathbf{y}}_l = (\tilde{y}_l(1), \ldots, \tilde{y}_l(n))^T$ for $l = 1, 2, \ldots, d$.

For $((\hat{\sigma}_0^2)^{new}, \hat{\boldsymbol{\rho}}^{new}, (\hat{\boldsymbol{\sigma}}^2)^{new})$, we take partial derivatives of Equation (11) with respect to $\sigma_0^2$, $\boldsymbol{\sigma}^2$ and $\boldsymbol{\rho}$, respectively, and set the equations to be zero:

$$\frac{\partial}{\partial \rho_l}\bar{\ell}(\boldsymbol{\Theta}) = \beta_0 + \beta_1\rho_l + \beta_2\rho_l^2 + \beta_3\rho_l^3 = 0, \tag{SM3.2}$$

$$\frac{\partial}{\partial \sigma_0^2}\bar{\ell}(\boldsymbol{\Theta}) = -\frac{nk}{2\sigma_0^2} - \frac{\text{tr}(\mathbf{Y}^T\hat{\mathbf{U}}_0^{\text{new}}\hat{\mathbf{Z}})}{\sigma_0^4} + \frac{\text{tr}(\mathbf{Y}^T\mathbf{Y}) + \sum_{l=1}^d\sum_{t=1}^n(s_l^2(t) + S_l(t))}{2\sigma_0^4} = 0, \tag{SM3.3}$$

$$\begin{aligned}\frac{\partial}{\partial \sigma_l^2}\bar{\ell}(\boldsymbol{\Theta}) &= -\frac{n}{2\sigma_l^2} + \frac{(1-\rho_l^2)s_l(1) + \sum_{t=2}^n(s_l(t) - \rho_l s_l(t-1))^2}{2\sigma_l^4} \\ &+ \frac{\sum_{t=1}^n S_l(t) + \rho_l^2\sum_{t=2}^{n-1} S_l(t) - 2\rho_l\sum_{t=1}^{n-1}\tilde{S}_l(t)}{2\sigma_l^4} = 0,\end{aligned} \tag{SM3.4}$$

where $\beta_0 = n\Big(\sum_{t=2}^n s_l(t-1)s_l(t) + \sum_{t=1}^{n-1}\tilde{S}_l(t)\Big)$, $\beta_1 = -\sum_{t=1}^n s_l^2(t) - \sum_{t=1}^n S_l(t) - n\sum_{t=2}^{n-1} s_l^2(t) - n\sum_{t=2}^{n-1} S_l(t)$, $\beta_2 = (2-n)(\sum_{t=2}^n s_l(t-1)s_l(t) + \sum_{t=1}^{n-1}\tilde{S}_l(t))$, $\beta_3 = (n-1)(\sum_{t=2}^{n-1} s_l^2(t) + \sum_{t=2}^{n-1} S_l(t))$, and the superscript "new" is omitted for simplicity.

Solving Equation (SM3.2) in $(-1,1)$ provides the updated estimation of $\rho_l$. We show that there is a unique root in $(-1,1)$ for this cubic equation. Consider a function of $\rho$ such that $h(\rho) = \beta_0 + \beta_1\rho_l + \beta_2\rho_l^2 + \beta_3\rho_l^3$. Since $\beta_3 = (n-1)(\sum_{t=2}^{n-1} s_l^2(t) + \sum_{t=2}^{n-1} S_l(t)) > 0$ for $n > 1$, $h(\rho) > 0$ as $\rho \to \infty$ and $h(\rho) < 0$ as $\rho \to -\infty$.

First we substitute $\rho = -1$:

$$
\begin{aligned}
h(-1) =&\beta_0 - \beta_1 + \beta_2 - \beta_3 \\
=&\sum_{t=1}^{n} s_l^2(t) + \sum_{t=1}^{n} S_l(t) + 2\sum_{t=2}^{n} s_l(t-1)s_l(t) + 2\sum_{t=1}^{n-1} \tilde{S}_l(t) + \sum_{t=2}^{n-1} s_l^2(t) + \sum_{t=2}^{n-1} S_l(t) \\
=&\left(\sum_{t=1}^{n-1} s_l^2(t) + 2\sum_{t=2}^{n} s_l(t-1)s_l(t) + \sum_{t=2}^{n} s_l^2(t)\right) \\
&+\left(\sum_{t=1}^{n-1} S_l(t) + 2\sum_{t=1}^{n-1} \tilde{S}_l(t) + \sum_{t=2}^{n} S_l(t)\right) \\
=&\sum_{t=1}^{n-1} (s_l(t) + s_l(t+1))^2 + \sum_{t=1}^{n-1} \mathbb{V}\left(z_l(t) + z_l(t+1) \mid \mathbf{Y}, \hat{\mathbf{\Theta}}\right) \\
>&0,
\end{aligned}
$$

where strict inequality is held as the second term is strictly larger than zero. This is because

$$
\begin{aligned}
&\mathbb{V}\left(z_l(t) + z_l(t+1) \mid \mathbf{Y}, \hat{\mathbf{\Theta}}\right) \\
=&\mathbb{V}\left(z_l(t) \mid \mathbf{Y}, \hat{\mathbf{\Theta}}\right) + \mathbb{V}\left(z_l(t+1) \mid \mathbf{Y}, \hat{\mathbf{\Theta}}\right) + 2\,\mathrm{Cov}\left(z_l(t), z_l(t+1) \mid \mathbf{Y}, \hat{\mathbf{\Theta}}\right) \\
\geq&\mathbb{V}\left(z_l(t) \mid \mathbf{Y}, \hat{\mathbf{\Theta}}\right) + \mathbb{V}\left(z_l(t+1) \mid \mathbf{Y}, \hat{\mathbf{\Theta}}\right) - 2\,\mathbb{V}\left(z_l(t) \mid \mathbf{Y}, \hat{\mathbf{\Theta}}\right)^{1/2} \mathbb{V}\left(z_l(t+1) \mid \mathbf{Y}, \hat{\mathbf{\Theta}}\right)^{1/2} \\
=&\left\{\mathbb{V}\left[z_l(t) \mid \mathbf{Y}, \hat{\mathbf{\Theta}}\right]^{1/2} - \mathbb{V}\left[z_l(t+1) \mid \mathbf{Y}, \hat{\mathbf{\Theta}}\right]^{1/2}\right\}^2
\end{aligned}
$$

where the last equation is due to

$$
\mathrm{Cov}[z_l(t), z_l(t+1) \mid \mathbf{Y}, \hat{\mathbf{\Theta}}] < \left(\mathbb{V}[z_l(t) \mid \mathbf{Y}, \hat{\mathbf{\Theta}}]\, \mathbb{V}[z_l(t+1) \mid \mathbf{Y}, \hat{\mathbf{\Theta}}]\right)^{1/2}.
$$

We only need to show there exists one $t$, $1 \leq t < n-1$,

$$
\left\{\mathbb{V}\left[z_l(t) \mid \mathbf{Y}, \hat{\mathbf{\Theta}}\right]^{1/2} - \mathbb{V}\left[z_l(t+1) \mid \mathbf{Y}, \hat{\mathbf{\Theta}}\right]^{1/2}\right\}^2 > 0.
$$

First, as $\hat{\sigma}_0^2 > 0$, we have $\mathbb{V}\left[z_l(t) \mid \mathbf{Y}, \hat{\mathbf{\Theta}}\right]^{1/2} > 0$. Second, as $\hat{\sigma}_l > 0$, we have

$$
\mathbb{V}\left[z_l(n) \mid \mathbf{Y}, \hat{\mathbf{\Theta}}\right]^{1/2} < \mathbb{V}\left[z_l(n-1) \mid \mathbf{Y}, \hat{\mathbf{\Theta}}\right]^{1/2}.
$$

These two facts lead to $\sum_{t=1}^{n-1} \mathbb{V}\left(z_l(t) + z_l(t+1) \mid \mathbf{Y}, \hat{\mathbf{\Theta}}\right) > 0$. Therefore, there exists at least one root in $(-\infty, -1)$.

Next we substitute $\rho = 1$:

$$
\begin{aligned}
h(1) =& \beta_0 + \beta_1 + \beta_2 + \beta_3 \\
=& -\sum_{t=1}^{n} s_l^2(t) - \sum_{t=1}^{n} S_l(t) + 2\sum_{t=2}^{n} s_l(t-1)s_l(t) + 2\sum_{t=1}^{n-1} \tilde{S}_l(t) - \sum_{t=2}^{n-1} s_l^2(t) - \sum_{t=2}^{n-1} S_l(t) \\
=& -\left(\sum_{t=1}^{n-1} s_l^2(t) - 2\sum_{t=2}^{n} s_l(t-1)s_l(t) + \sum_{t=2}^{n} s_l^2(t)\right) \\
& -\left(\sum_{t=1}^{n-1} S_l(t) - 2\sum_{t=1}^{n-1} \tilde{S}_l(t) + \sum_{t=2}^{n} S_l(t)\right) \\
=& -\sum_{t=1}^{n-1} (s_l(t) - s_l(t+1))^2 - \sum_{t=1}^{n-1} \mathbb{V}\left(z_l(t) - z_l(t+1) \mid \mathbf{Y}, \hat{\boldsymbol{\Theta}}\right) < 0.
\end{aligned}
$$

The strict inequality is due to $\hat{\sigma}_0^2 > 0$ and $\hat{\sigma}_l^2 > 0$. Hence, there exists at least one root in $(1, \infty)$.

Since $h(-1) > 0$ and $h(1) < 0$, by the intermediate value theorem, there exists at least one root in $\hat{\rho} \in (-1, 1)$ such that $h(\hat{\rho}) = 0$. Furthermore, since $h(\rho)$ is cubic, it has at most three roots, with one root in $(-\infty, -1)$, one in $(1, \infty)$, and the root in $(-1, 1)$. Hence, for Equation (SM3.2), the root in $(-1, 1)$ exists and is unique.

Furthermore, solving Equations (SM3.3) and (SM3.4) gives the analytical expression of $(\hat{\sigma}_0^2)^{\text{new}}$ and $(\hat{\boldsymbol{\sigma}}^2)^{\text{new}}$ which are given in Equation (17) and Equation (19), respectively.

Now we prove that $((\hat{\sigma}_0^2)^{\text{new}}, (\hat{\boldsymbol{\sigma}}^2)^{\text{new}})$ maximize Equation (11) by showing that the second derivative is negative at the updated estimators.

$$
\begin{aligned}
& \frac{\partial^2}{\partial(\sigma_0^2)^2} \bar{\ell}(\boldsymbol{\Theta})\Big|_{\sigma_0^2 = (\hat{\sigma}_0^2)^{\text{new}}} \\
&= \frac{1}{2(\hat{\sigma}_0^6)^{\text{new}}} \left( -\operatorname{tr}(\mathbf{Y}^T\mathbf{Y}) - \operatorname{tr}(\hat{\mathbf{Z}}^T\hat{\mathbf{Z}}) + 2\operatorname{tr}(\mathbf{Y}^T\hat{\mathbf{U}}_0^{\text{new}}\hat{\mathbf{Z}})) - \sum_{l=1}^{d}\sum_{t=1}^{n} S_l(t) \right).
\end{aligned}
$$

Since $-\operatorname{tr}(\mathbf{Y}^T\mathbf{Y}) - \operatorname{tr}(\hat{\mathbf{Z}}^T\hat{\mathbf{Z}}) + 2\operatorname{tr}(\mathbf{Y}^T\hat{\mathbf{U}}_0^{\text{new}}\hat{\mathbf{Z}})) = -\operatorname{tr}\left(\|\mathbf{Y} - \hat{\mathbf{U}}_0^{\text{new}}\hat{\mathbf{Z}}\|_F^2\right) < 0$ for $\mathbf{Y} \neq \hat{\mathbf{U}}_0^{\text{new}}\hat{\mathbf{Z}}$, $S_l(t) \geq 0$ for any $l, t$, and $(\hat{\sigma}_0^2)^{\text{new}} > 0$, the second derivative of $\sigma_0^2$ at $(\hat{\sigma}_0^2)^{\text{new}}$ is negative. Therefore, $(\hat{\sigma}_0^2)^{\text{new}}$ maximizes Equation (11).

Beside, since

$$
\frac{\partial^2}{\partial(\sigma_l^2)^2} \bar{\ell}(\boldsymbol{\Theta})\Big|_{\sigma_l^2 = (\hat{\sigma}_l^2)^{\text{new}}} = -\frac{n}{2(\hat{\sigma}_l^4)^{\text{new}}} < 0, \qquad \blacksquare
$$

$(\hat{\sigma}_l^2)^{\text{new}}$ maximizes Equation (11).

**SM3.5. EM algorithm with known $\mathbf{U}_0$ and $\sigma_0^2$.** When employing our FMOU model in deformation data inversion, the loading matrix $\mathbf{U}_0$ is derived from the matrix of Green's

function, and the noise intensity $\sigma_0^2$ is usually available as the observation uncertainty. In this case, we only need to estimate $\boldsymbol{\rho}$ and $\boldsymbol{\sigma}^2$. The MMLEs of the parameters can be obtained by maximizing the marginal likelihood of $\mathbf{Y}$:

$$\begin{aligned}(\boldsymbol{\rho}^{\text{MMLE}}, (\boldsymbol{\sigma}^2)^{\text{MMLE}}) &= \underset{\boldsymbol{\rho},\boldsymbol{\sigma}^2}{\text{argmax}}\, p(\mathbf{Y} \mid \boldsymbol{\rho}, \boldsymbol{\sigma}^2) \\ &= \underset{\boldsymbol{\rho},\boldsymbol{\sigma}^2}{\text{argmax}} \int p(\mathbf{Y} \mid \mathbf{Z}, \mathbf{U}_0, \sigma_0^2, \boldsymbol{\rho}, \boldsymbol{\sigma}^2) p(\mathbf{Z} \mid \boldsymbol{\rho}, \boldsymbol{\sigma}^2) d\mathbf{Z},\end{aligned}$$

The joint log-likelihood of $(\mathbf{Y}, \mathbf{Z} \mid \mathbf{U}_0, \sigma_0^2, \boldsymbol{\rho}, \boldsymbol{\sigma}^2)$ can be written as:

$$\begin{aligned}\ell(\boldsymbol{\rho}, \boldsymbol{\sigma}^2) &= \log\left(p(\mathbf{Y}, \mathbf{Z} \mid \mathbf{U}_0, \sigma_0^2, \boldsymbol{\rho}, \boldsymbol{\sigma}^2)\right) \\ &= \tilde{C} + \sum_{l=1}^{d} \Big( \frac{2\mathbf{z}_l^T \tilde{\mathbf{y}}_l - \mathbf{z}_l^T \mathbf{z}_l}{2\sigma_0^2} - \frac{\log|\boldsymbol{\Sigma}_l|}{2} - \frac{\mathbf{z}_l^T \boldsymbol{\Sigma}_l^{-1} \mathbf{z}_l}{2} \Big),\end{aligned} \tag{SM3.5}$$

where $\tilde{C} = -\frac{(nk+nd)}{2}\log(2\pi) - \frac{nk}{2}\log(\sigma_0^2) - \frac{\text{tr}(\mathbf{Y}^T\mathbf{Y})}{2\sigma_0^2}$ is constant since $\sigma_0^2$ is known, and $\tilde{\mathbf{Y}} = \mathbf{U}_0^T \mathbf{Y} = [\tilde{\mathbf{y}}_1, \ldots, \tilde{\mathbf{y}}_d]^T$.

In the E-step, we take the expectation of Equation (SM3.5) with respect to the conditional distribution of $\mathbf{Z}$ based on the current estimation of $(\hat{\boldsymbol{\rho}}, \hat{\boldsymbol{\sigma}}^2)$ and observations $\mathbf{Y}$:

$$\begin{aligned}\bar{\ell}(\boldsymbol{\rho}, \boldsymbol{\sigma}^2) :&= \mathbb{E}_{\mathbf{Z}|\mathbf{Y},\mathbf{U}_0,\sigma_0^2,\hat{\boldsymbol{\rho}},\hat{\boldsymbol{\sigma}}^2}[\ell(\boldsymbol{\rho}, \boldsymbol{\sigma}^2)] \\ &= \tilde{C} - \frac{1}{2}\sum_{l=1}^{d} \log|\boldsymbol{\Sigma}_l| + \frac{\sum_{l=1}^{d} \mathbb{E}_{\mathbf{Z}|\mathbf{Y},\mathbf{U}_0,\sigma_0^2,\hat{\boldsymbol{\rho}},\hat{\boldsymbol{\sigma}}^2}[\mathbf{z}_l^T \tilde{\mathbf{y}}_l]}{\sigma_0^2} - \sum_{l=1}^{d} \frac{\mathbb{E}_{\mathbf{Z}|\mathbf{Y},\mathbf{U}_0,\sigma_0^2,\hat{\boldsymbol{\rho}},\hat{\boldsymbol{\sigma}}^2}[\mathbf{z}_l^T \mathbf{z}_l]}{2\sigma_0^2} \\ &\quad - \sum_{l=1}^{d} \frac{\mathbb{E}_{\mathbf{Z}|\mathbf{Y},\mathbf{U}_0,\sigma_0^2,\hat{\boldsymbol{\rho}},\hat{\boldsymbol{\sigma}}^2}[\mathbf{z}_l^T \boldsymbol{\Sigma}_l^{-1} \mathbf{z}_l]}{2}\end{aligned} \tag{SM3.6}$$

$$\begin{aligned}&= \tilde{C} - \frac{1}{2}\sum_{l=1}^{d} \log|\boldsymbol{\Sigma}_l| + \frac{\sum_{l=1}^{d} \hat{\mathbf{z}}_l^T \tilde{\mathbf{y}}_l}{\sigma_0^2} - \sum_{l=1}^{d} \frac{\hat{\mathbf{z}}_l^T \hat{\mathbf{z}}_l + \text{tr}[\sigma_0^2 \hat{\boldsymbol{\Sigma}}_l (\hat{\boldsymbol{\Sigma}}_l + \sigma_0^2 \mathbf{I}_n)^{-1}]}{2\sigma_0^2} \\ &\quad - \sum_{l=1}^{d} \frac{\hat{\mathbf{z}}_l^T \boldsymbol{\Sigma}_l^{-1} \hat{\mathbf{z}}_l + \text{tr}[\sigma_0^2 \boldsymbol{\Sigma}_l^{-1} \hat{\boldsymbol{\Sigma}}_l (\hat{\boldsymbol{\Sigma}}_l + \sigma_0^2 \mathbf{I}_n)^{-1}]}{2}.\end{aligned} \tag{SM3.7}$$

To estimate $\boldsymbol{\rho}$ and $\boldsymbol{\sigma}^2$, one only needs to force $\hat{\mathbf{U}}_0^{\text{new}} \equiv \mathbf{U}_0$ and $(\hat{\sigma}_0^2)^{\text{new}} \equiv \sigma_0^2$ throughout the iterations. The analytical forms of updating $\rho_l$ and $\sigma_l^2$ are provided in Equations (18) and (19).

## SM4. Summary of other methods.

**SM4.1. The dynamic mode decomposition.** The exact dynamic mode decomposition (DMD) algorithm from [SM12] is summarized below.

1. Compute the singular value decomposition (SVD) of $\mathbf{Y}_{1:n-1} = \bar{\mathbf{U}}\bar{\mathbf{D}}\bar{\mathbf{V}}^T$ and keep the first $d$ ($d \le \min(k, n)$) largest singular values and the associated singular vectors, denoted as $\bar{\mathbf{U}}_0$, $\bar{\mathbf{D}}_0$ and $\bar{\mathbf{V}}_0$. Hence, $\bar{\mathbf{A}}$ in Equation (24)

2. Project $\bar{\mathbf{A}}$ onto the column space of $\bar{\mathbf{U}}_0$ and form the matrix $\tilde{\mathbf{A}} = \bar{\mathbf{U}}_0^T \bar{\mathbf{A}} \bar{\mathbf{U}}_0$.
3. Let $(\bar{\lambda}_l, \bar{\boldsymbol{\omega}}_l)$, $l = 1, 2, \ldots, d$, be the eigenvalue-eigenvector pair of $\tilde{\mathbf{A}}$. Then $\bar{\lambda}_l$ is the eigenvalue of $\bar{\mathbf{A}}$, with the corresponding eigenvector $\bar{\boldsymbol{\varphi}}_l = \mathbf{Y}_{2:n} \bar{\mathbf{V}}_0 \bar{\mathbf{D}}_0^{-1} \bar{\boldsymbol{\omega}}_l / \bar{\lambda}_l$.

In DMD, one typically sets $\hat{d}$ as the number of leading eigenvalues that account for at least 99% of the total variance.

**SM4.2. The network inversion filter.** The network inversion filter (NIF) proposed by [SM11] is a routinely used approach for inverse estimation of geodetic data. The slips of interest are assumed to be a linear combination of $d$ orthogonal basis functions in Equation (2) with coefficient vectors $\tilde{\mathbf{z}}_l = [\tilde{z}_l(1), \ldots, \tilde{z}_l(n)]^T$ constructed by $\tilde{z}_l(t) = v_l t + W_l(t)$ for $l = 1, \ldots, d$ and $t = 1, \ldots, n$, where $v_l$ is a time-independent velocity and $W_l(t) = \int_0^t B(t')dt'$ is an integrated Brownian motion with a scale parameter $\alpha$. The orthogonal basis functions are chosen as $\mathbf{U}_0 \boldsymbol{\Lambda}_0$, where the $k \times d$ orthogonal matrix $\mathbf{U}_0$ and the $d \times d$ diagonal matrix $\boldsymbol{\Lambda}_0$ contain the first $d$ eigenvectors and eigenvalues of $\mathbf{G}\mathbf{G}^T$, respectively. Thus $\boldsymbol{\Lambda}_0 = \mathbf{D}_0^2$. For equally spaced time points, the model below is assumed in NIF for GPS measurements

$$
\begin{aligned}
\mathbf{y}(t) &= \mathbf{U}_0 \boldsymbol{\Lambda}_0 \mathbf{X}(t) + \boldsymbol{\epsilon}(t), \quad \boldsymbol{\epsilon}(t) \sim \mathcal{MN}(\mathbf{0}, \sigma_0^2 \mathbf{I}_k), \\
W_l(t) &= W_l(t-1) + \dot{W}_l(t-1) + \omega_l(t), \quad \omega_l(t) \sim \mathcal{N}\left(0, \frac{\alpha^2}{3}\right), \\
\dot{W}_l(t) &= \dot{W}_l(t-1) + \dot{\omega}_l(t), \quad \dot{\omega}_l(t) \sim \mathcal{N}(0, \alpha^2),
\end{aligned}
$$

where the state vector $\mathbf{X}(t) = [v_1 t + W_1(t), \ldots, v_d t + W_d(t)]^T$, $\dot{W}_l(t)$ represents the derivative of $W_l(t)$, and $\mathrm{Cov}(\omega_l(t), \dot{\omega}_l(t)) = \frac{\alpha^2}{2}$, for $l = 1, \ldots, d$. When using the KF for computing the likelihood function, one needs to directly invert some $k \times k$ matrices in each step, which can be computationally expensive for large $k$, as the overall computational complexity of NIF is $\mathcal{O}(\min(k^2 k', k(k')^2)) + \mathcal{O}(M_0 n k^3)$, where $M_0$ is the number of optimization steps taken by NIF. In comparison, the computational operation of our EM algorithm for the FMOU model using a given Green's function only requires $\mathcal{O}(\min(k^2 k', k(k')^2)) + \mathcal{O}(Mknd)$ operations. As the second term is dominating the computation, the FMOU is at the order of $k^2/d$ times faster than the NIF in each iteration of the optimization.

**SM4.3. Modified NIF applied for the 2011 Cascadia data.** In the modified NIF proposed in [SM1], the GPS data in Cascadia at any time $t$ follows

$$
\mathbf{y}(t) = \tilde{\mathbf{G}} \tilde{\mathbf{z}}_s(t) + \boldsymbol{\epsilon}(t) = \mathbf{G} \mathbf{z}_s(t) + \begin{pmatrix} \mathbf{I}_2 \\ \vdots \\ \mathbf{I}_2 \end{pmatrix} \mathbf{f}_2 + \boldsymbol{\epsilon}(t). \tag{SM4.1}
$$

Here $\mathbf{f}_2 = (f_E, f_N)^T$ denotes the reference frame motions in the East-West and North-South directions, assumed to follow $\mathcal{MN}(\mathbf{0}, \sigma_f^2 \mathbf{I}_2)$, where $\sigma_f^2$ measures the amplitude of external global motions. One can rewrite the modified NIF model as a dynamic linear model:

$$
\mathbf{y}(t) = \mathbf{H}(t) \mathbf{X}(t) + \boldsymbol{\epsilon}(t) \quad \boldsymbol{\epsilon}(t) \sim \mathcal{MN}(\mathbf{0}, \sigma_0^2 \mathbf{I}_k), \tag{SM4.2}
$$

$$
\mathbf{X}(t) = \mathbf{T}(t) \mathbf{X}(t-1) + \boldsymbol{\delta}(t), \quad \boldsymbol{\delta}(t) \sim \mathcal{MN}(\mathbf{0}, \boldsymbol{\Omega}(t)). \tag{SM4.3}
$$

The terms in Equation (SM4.2) and (SM4.3) are specified as follows.

1. The latent states $\mathbf{X}(t)$ includes slips and slip rates at time $t$:

$$\mathbf{X}(t) = [z_s(\boldsymbol{\xi}_1, t), \dot{z}_s(\boldsymbol{\xi}_1, t), ..., z_s(\boldsymbol{\xi}_{k'}, t), \dot{z}_s(\boldsymbol{\xi}_{k'}, t), \mathbf{f}_2]^T \in \mathbb{R}^{2k'+2},$$

where $\dot{z}_s(\boldsymbol{\xi}_h, t)$ represents the slip rate at $\boldsymbol{\xi}_h$ and time $t$, for $h = 1, \ldots, k'$ and $t = 1, \ldots, n$.

2. $\mathbf{H}(t) = \left(\mathbf{G}^*, \mathbf{I}_k\right) \in \mathbb{R}^{k\times(k+2k')}$, where $\mathbf{G}^* = \mathbf{G}\begin{pmatrix} 1 & 0 & 1 & 0 & 1 & \cdots & 1 & 0 \\ 1 & 0 & 1 & 0 & 1 & \cdots & 1 & 0 \\ \vdots & & & \vdots & & \vdots & & \vdots \\ 1 & 0 & 1 & 0 & 1 & \cdots & 1 & 0 \end{pmatrix}_{k'\times 2k'}$ is a matrix of Green's function calculated for the Cascadia region.

3. $\mathbf{T}(t) = \begin{pmatrix} \mathbf{T}^0(t) & & & \\ & \ddots & & \\ & & \mathbf{T}^0(t) & \\ & & & \mathbf{0} \end{pmatrix} \in \mathbb{R}^{2k'+1}$, where $\mathbf{T}^0(t) = \begin{pmatrix} 1 & 1 \\ 0 & 1 \end{pmatrix}$.

4. $\boldsymbol{\Omega}(t) = \begin{pmatrix} \boldsymbol{\Omega}^0(t) & & & \\ & \ddots & & \\ & & \boldsymbol{\Omega}^0(t) & \\ & & & \sigma_f^2\mathbf{I}_2 \end{pmatrix}$, where $\boldsymbol{\Omega}^0(t) = \begin{pmatrix} \frac{\alpha^2}{3} & \frac{\alpha^2}{2} \\ \frac{\alpha^2}{2} & \alpha^2 \end{pmatrix}$.

The parameter $\alpha$ and $\sigma_f^2$ can be estimated by the MLE, where KF is used to compute the likelihood function and RTS smoother is used for computing the posterior distribution of the slip. Due to the high computational cost of inverting the covariance matrices at each time point, only a small number of parameter values at a grid is computed in modified NIF to approximate MLE.

As the dimension of state spaces depends entirely on $k$ and $k'$, the MATLAB code proposed in [SM1] requires more time for the computation compared to both the FMOU model and NIF model due to matrix inversions of a $k \times k$ matrix during forward filtering, and a $(2(k'+1)) \times (2(k'+1))$ matrix during backward smoothing. The Woodbury matrix identity can be used to simplify the computation cost of the modified NIF so that it is closer to the NIF model.

## SM5. Supplement to simulation results.

### SM5.1. Uncertainty quantification of the predictive signal and slip.

We consider two additional criteria to evaluate the model, including the average length of the 95% posterior credible intervals of the signal, i.e. the mean of the observation, and the slip ($\mathrm{L}^m(95\%)$, $\mathrm{L}^s(95\%)$), and the proportion of the signal and the slip covered by the 95% posterior credible

| Estimated $d$ | $\sigma_0^2 = 1$ | | | $\sigma_0^2 = 2$ | | |
|---|---|---|---|---|---|---|
| | $n = 100$ | $n = 200$ | $n = 400$ | $n = 100$ | $n = 200$ | $n = 400$ |
| FMOU | **0.41** | **0.35** | **0.33** | **0.62** | **0.53** | **0.44** |
| DMD | 0.71 | 0.67 | 0.65 | 0.91 | 0.83 | 0.80 |
| LY1 | 1.3 | 1.1 | 0.71 | 2.0 | 1.5 | 1.0 |
| LY5 | 1.7 | 0.95 | 0.65 | 2.0 | 1.4 | 1.2 |

**Table SM1**

*Average of $RMSE_m$ over $N$ simulated configurations in Experiment 2 with $d$ estimated by 4 different methods.*

intervals ($\mathrm{P}^m(95\%)$, $\mathrm{P}^s(95\%)$):

$$\mathrm{L}^m(95\%) = \frac{1}{kn}\sum_{t=1}^{n}\sum_{i=1}^{k}\text{length}\{\mathrm{CI}_{i,t}^m(95\%)\}, \tag{SM5.1}$$

$$\mathrm{L}^s(95\%) = \frac{1}{k'n}\sum_{t=1}^{n}\sum_{h=1}^{k'}\text{length}\{\mathrm{CI}_{h,t}^s(95\%)\}, \tag{SM5.2}$$

$$\mathrm{P}^m(95\%) = \frac{1}{kn}\sum_{t=1}^{n}\sum_{i=1}^{k}1_{(\mathbf{m}(t)))_i \in \mathrm{CI}_{i,t}^m(95\%)}, \tag{SM5.3}$$

$$\mathrm{P}^s(95\%) = \frac{1}{k'n}\sum_{t=1}^{n}\sum_{h=1}^{k'}1_{(z_{s,h}(t)) \in \mathrm{CI}_{h,t}^s(95\%)}, \tag{SM5.4}$$

where the superscript 'm' and 's' denote the mean and slip, respectively.

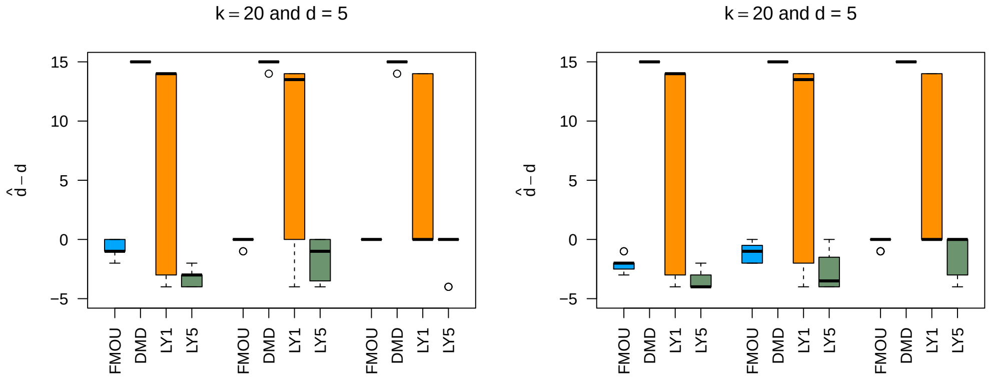


**Figure SM1.** *Differences between the selected number of factors and the truth by different methods in Experiment 2. In each subfigure, the first 4, middle 4, and the last 4 boxes are based on $n = 100$, $n = 200$, and $n = 300$, respectively. The noise variance is $\sigma_0^2 = 1$ and $\sigma_0^2 = 2$ for the left and right subfigures, respectively.*

**SM5.2. Additional results in Experiment 2 .** In Figure SM1, we plot the difference between the estimated number of latent factor $\hat{d}$ and the true latent factor using four different

| True d | $\sigma_0^2 = 1$ | | | $\sigma_0^2 = 2$ | | |
|---|---|---|---|---|---|---|
| | $n = 100$ | $n = 200$ | $n = 400$ | $n = 100$ | $n = 200$ | $n = 400$ |
| $\mathrm{L}^m(95\%)$ | 1.2 | 1.2 | 1.2 | 1.5 | 1.5 | 1.5 |
| $\mathrm{P}^m(95\%)$ | 88% | 91% | 93% | 87% | 90% | 92% |
| $\mathrm{SD}_{signal}$ | 5.1 | 2.2 | 2.9 | 5.1 | 2.2 | 2.9 |
| Estimated d | $\sigma_0^2 = 1$ | | | $\sigma_0^2 = 2$ | | |
| | $n = 100$ | $n = 200$ | $n = 400$ | $n = 100$ | $n = 200$ | $n = 400$ |
| $\mathrm{L}^m(95\%)$ | 1.1 | 1.2 | 1.2 | 1.1 | 1.3 | 1.4 |
| $\mathrm{P}^m(95\%)$ | 82% | 90% | 93% | 64% | 77% | 90% |
| $\mathrm{SD}_{signal}$ | 5.1 | 2.2 | 2.9 | 5.1 | 2.2 | 2.9 |

**Table SM2**

*The average lengths of 95% posterior credible intervals, the percentages of the signal covered by the intervals from FMOU, and the standard deviation of signals ($SD_{signal}$) for Experiment 3.*

methods. The estimation accuracy based on IC, LY1 and LY5 improves with larger sample sizes. Among these methods, IC consistently outperforms the other methods in accuracy across all configurations. Table SM1 displays the $\mathrm{RMSE}_m$ by the four methods using the estimated number of latent factors. The FMOU method achieves the most accurate estimation of the signal from noise observations.

Table SM2 summarizes the average length and proportion of the signal covered in 95% posterior credible intervals of FMOU. The lengths of the intervals are relatively short compared to the standard deviation of the signal, indicating precise estimation. Note that this simulation represents a challenging scenario, as the model contains a large number of parameters that cannot be integrated out, and the variance of noise is relatively large. Consequently, the true values covered by the 95% credible interval are shorter than 95% for a small sample size. When the sample size grows to moderately large, the percentage of the true outputs covered by the 95% posterior credible interval increases to be close to 95%.

**SM5.3. Additional results in Experiment 3.** Table SM3 shows the average length of the 95% posterior credible intervals and the percentage of the signal covered in the 95% posterior credible intervals. The length of the 95% posterior credible intervals is short compared to the standard deviation of the signal, indicating the method is precise. In both the linear diffusion and Branin function examples, the percentage of the signal covered in the 95% posterior credible interval is smaller than 95%, particularly when the noise variance is large. This discrepancy arises because the signal is governed by a smooth process, while the FMOU process is not differentiable.

**SM5.4. Additional results in Experiment 4 .** In Experiment 4, we assess the accuracy of $\hat{d}$ selected by three approaches. First, assuming $\sigma_0^2$ is unknown, we apply the IC criterion based on the left singular vectors of observations and the known factor loading matrix $\mathbf{U}$. We also employ the variance matching (VM) method to estimate the number of factors. Since $d$ can take values from 1 to $k$, estimating the noise levels for all possible values of $d$ can be slow when $k$ is large. As $\hat{\sigma}_0^2(d)$ is approximately nonincreasing over $d$, we use the binary search

| | Linear diffusion | | | Branin function | | |
|---|---|---|---|---|---|---|
| | $\sigma_0^2 = 0.0001$ | $\sigma_0^2 = 0.0025$ | $\sigma_0^2 = 0.09$ | $\sigma_0^2 = 1$ | $\sigma_0^2 = 25$ | $\sigma_0^2 = 400$ |
| $\mathrm{L}^m(95\%)$ | 0.0046 | 0.016 | 0.038 | 0.35 | 1.5 | 4.2 |
| $\mathrm{P}^m(95\%)$ | 75% | 72% | 42% | 80% | 77% | 67% |
| $\mathrm{SD}_{signal}$ | 0.30 | 0.30 | 0.30 | 52 | 52 | 52 |

Table SM3

*The average lengths of 95% posterior credible intervals, the percentages of the samples covered by the interval from FMOU, and the standard deviation of signals ($SD_{signal}$) for Experiment 3.*

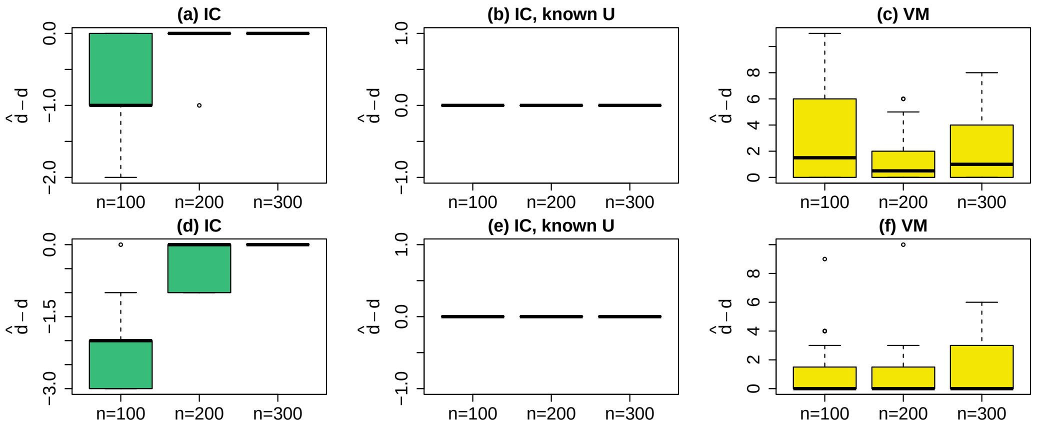


**Figure SM2.** *Difference between $\hat{d}$ and $d$ under different combinations of parameters in Experiment 4. Three approaches are compared: 1) the 'IC' method denotes the IC criterion with factor loading matrix constructed by left singular vectors of observations; 2) the 'IC, known U' method denotes the IC criterion using the known* $\mathbf{U}$ *as factor loading matrix; 3) the 'VM' method denotes the variance matching method. The results for scenarios with $(k = 25, k' = 150, d = 6)$ are shown in panels (a)-(c), and the results for scenarios with $(k = 32, k' = 100, d = 8)$ are shown in panels (d)-(f).*

algorithm [SM3] to find a $d$ that yields a $\hat{\sigma}_0^2$ closest to the known noise level. The results are summarized in Figure SM2. The IC criterion with the known factor loading matrix accurately estimates $d$ for both small and moderately large sample sizes. The VM method tends to slightly overestimate the number of factors in some simulation scenarios. Note that the goal of the VM is to select a model to approximate the signal. We found that the selected models with a slightly larger number of factors and more parameters tend to have better performance when the model is misspecified.

Figure SM3 compares $\mathrm{RMSE}_m$ with different methods of selecting $d$. The predictive accuracy of the signal aligns with the trends observed in Figure SM2, where all methods improve as the sample size increases. Among these methods, the VM and the IC criterion with a known $\mathbf{U}$ are more precise than the other approaches.

As shown in Table SM4 and SM5, the FMOU method provides relatively short 95% posterior credible intervals for both signals and slips, indicating precise estimation. The proportion of the samples covered in 95% of the posterior credible interval is close to 95% when the sample size is moderately large.

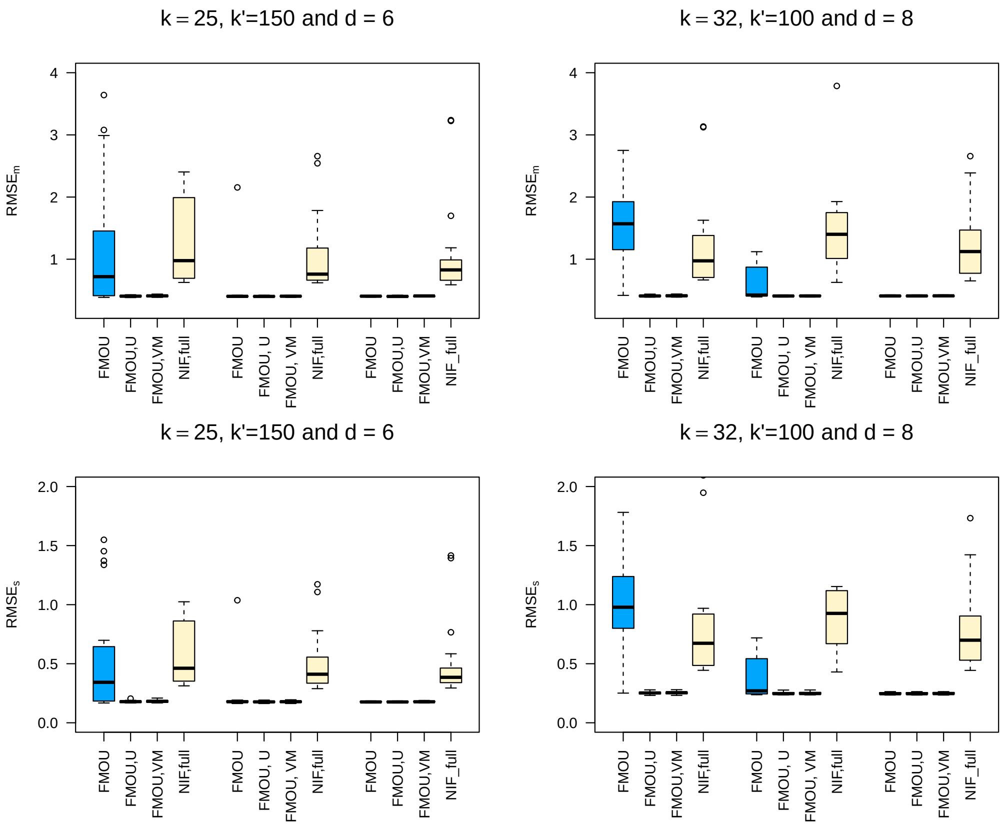


**Figure SM3.** *Box plots of* $RMSE_m$ *and* $RMSE_s$ *from 4 methods in Experiment 4. 1) 'FMOU': the estimated latent factor,* $\hat{d}$ *is selected by IC with factor loading matrix given by left singular vectors of observations. 2) 'FMOU, U':* $\hat{d}$ *selected by IC with a known factor loading* $\mathbf{U}$*; 3) 'FMOU, VM': d is estimated by variance matching; 4) 'NIF,full': NIF with full rank* $(d = k)$*. In each subfigure, the first 4, middle 4, and the last 4 boxes are based on* $n = 100$*,* $n = 200$ *and* $n = 300$*, respectively.*

**SM5.5. Additional results in Experiment 5.** Table SM6 provides the average length of the 95% posterior credible intervals of signals and slips by FMOU, and the percentages of the truth covered by the intervals for Experiment 5. The percentage of the signal covered by the interval is close to 95%, yet the percentage of the slip covered by the interval is smaller than 95%. This is because we only have 88 time points which are small, and the signal is misspecified. Obtaining more observations and extending the FMOU model with differentiable latent processes can increase the percentage of true slips covered by the model.

**SM6. Data preprocessing and model fitting for the Cascadia data.** The original observations, denoted as $\mathbf{y}^*(\mathbf{x}_i, t) \in \mathbb{R}^2$, represent the measurements in East-West and North-South directions at the $i$th GPS station and time point $t$, for $i = 1, \ldots, 100$, $t = 1, \ldots, 88$ indicating the total of $k = 100$ GPS stations and $n = 88$ days of observations. As identified by [SM2], the observed data include internal signals related to plate convergence, which are at a scale comparable to the slip-related signals. Following [SM2, SM1], we first remove the seasonal

| true d | $k=25, k'=150, d=6$ | | | $k=32, k'=100, d=8$ | | |
|---|---|---|---|---|---|---|
| | $n=100$ | $n=200$ | $n=300$ | $n=100$ | $n=200$ | $n=300$ |
| $\mathrm{L}^m(95\%)$ | 1.5 | 1.5 | 1.5 | 1.6 | 1.6 | 1.6 |
| $\mathrm{P}^m(95\%)$ | 95% | 95% | 95% | 95% | 95% | 95% |
| $\mathrm{SD}_{signal}$ | 2.4 | 2.5 | 2.4 | 3.6 | 2.7 | 2.6 |
| Estimated d | $k=25, k'=150, d=6$ | | | $k=32, k'=100, d=8$ | | |
| | $n=100$ | $n=200$ | $n=300$ | $n=100$ | $n=200$ | $n=300$ |
| $\mathrm{L}^m(95\%)$ | 1.6 | 1.5 | 1.5 | 1.6 | 1.6 | 1.6 |
| $\mathrm{P}^m(95\%)$ | 69% | 92% | 95% | 45% | 84% | 95% |
| $\mathrm{SD}_{signal}$ | 2.4 | 2.5 | 2.4 | 3.6 | 2.7 | 2.6 |

Table SM4

*The average lengths of the 95% posterior credible intervals, the percentages of the signal covered by the intervals from FMOU, and the standard deviation of the signals ($SD_{signal}$) for Experiment 4. IC is used for estimating the number of factors d.*

| true d | $k=25, k'=150, d=6$ | | | $k=32, k'=100, d=8$ | | |
|---|---|---|---|---|---|---|
| | $n=100$ | $n=200$ | $n=300$ | $n=100$ | $n=200$ | $n=300$ |
| $\mathrm{L}^s(95\%)$ | 0.67 | 0.66 | 0.66 | 0.95 | 0.95 | 0.95 |
| $\mathrm{P}^s(95\%)$ | 95% | 95% | 95% | 95% | 95% | 95% |
| $\mathrm{SD}_{slip}$ | 1.1 | 1.1 | 1.0 | 2.4 | 1.7 | 1.6 |
| Estimated d | $k=25, k'=150, d=6$ | | | $k=32, k'=100, d=8$ | | |
| | $n=100$ | $n=200$ | $n=300$ | $n=100$ | $n=200$ | $n=300$ |
| $\mathrm{L}^s(95\%)$ | 0.68 | 0.67 | 0.66 | 0.95 | 0.94 | 0.95 |
| $\mathrm{P}^s(95\%)$ | 68% | 92% | 95% | 45% | 84% | 95% |
| $\mathrm{SD}_{slip}$ | 1.1 | 1.1 | 1.0 | 2.4 | 1.7 | 1.6 |

Table SM5

*The average lengths of the 95% posterior credible intervals of the slips by FMOU, the true slip covered by the intervals, and the standard deviation of the slip ($SD_{slip}$) in Experiment 4. IC is used for estimating the number of factors d.*

components and get the processed data $\mathbf{y}(\mathbf{x}_i, t)$ by

$$\mathbf{y}(\mathbf{x}_i,t) = \mathbf{y}^*(\mathbf{x}_i,t) - \mathbf{c}_1 t - \mathbf{c}_2 sin(2\pi t) - \mathbf{c}_3 cos(2\pi t) - \mathbf{c}_4 sin(4\pi t) - \mathbf{c}_5 cos(4\pi t), \tag{SM6.1}$$

where $\mathbf{c}_1 = (c_{1,E}, c_{1,N})^T$ represents the secular velocity and $\mathbf{c}_2 = (c_{2,E}, c_{2,N})^T$, $\mathbf{c}_3 = (c_{3,E}, c_{3,N})^T$, $\mathbf{c}_4 = (c_{4,E}, c_{4,N})^T$, $\mathbf{c}_5 = (c_{5,E}, c_{5,N})^T$ represent the rates of four seasonal components in East-West and North-South directions. After obtaining $\mathbf{y}(t) = [\mathbf{y}^T(\mathbf{x}_1,t), \mathbf{y}^T(\mathbf{x}_2,t), \ldots, \mathbf{y}^T(\mathbf{x}_{100},t)]^T$ by Equation (SM6.1) for $t = 1, \ldots, 88$, we impute 15% of missing values using a Gaussian process model with an exponential covariance function separately for each station. The parameters are estimated by the MLE. We use the `FastGaSP R` package [SM5] to compute these predictive distributions and obtain posterior samples of the missing observations for imputa-

| | $L^m(95\%)$ | $P^m(95\%)$ | $SD_{signal}$ | $L^s(95\%)$ | $P^s(95\%)$ | $SD_{slip}$ |
|---|---|---|---|---|---|---|
| $\sigma_0^2 = 0.01^2$ | 0.014 | 92% | 0.19 | 0.25 | 50% | 0.85 |
| $\sigma_0^2 = 0.05^2$ | 0.044 | 90% | 0.19 | 0.51 | 61% | 0.85 |
| $\sigma_0^2 = 0.2^2$ | 0.12 | 89% | 0.19 | 0.87 | 73% | 0.85 |

**Table SM6**

*The average length of the 95% posterior credible intervals of signals by FMOU, the percentages of the samples covered by the intervals, and standard deviation of the signals and slips in Experiment 4.*

tion.

In the Cascadia dataset, the measurement noise variance are provided. As the noise variance at each location and time point is approximately the same, we use the average to estimate the variance of the noise in observations. We implement the variance matching method with binary search, described in Equation (22) to estimate the number of latent processes, $\hat{d} = 30$, in the FMOU model.

To compute the proportion of tremors detected by the large slip rate and the total areas containing a large slip rate shown in Figure 9, we partition the Cascadia subduction zone into 2,280 grids of equal area, with the temporal domain segmented into 16 intervals, each spanning 5 days. Given a threshold, we identify grids containing stations with larger average slip rates in 5 consecutive days. These grids are flagged as potential anomalies, and we count the number of grids having high slip rates. The proportion of identified tremors is defined as the ratio of grids containing both tremors and potential anomalies to the total number of grids with tremors.

Figure SM4 shows the estimated slip rates from FMOU, NIF and the modified NIF over other periods, in addition to Figure 10. The results are consistent with the findings discussed in the manuscript.

## REFERENCES

[1] N. M. Bartlow, S. Miyazaki, A. M. Bradley, and P. Segall, *Space-time correlation of slip and tremor during the 2009 cascadia slow slip event*, Geophysical Research Letters, 38 (2011).
[2] C. DeMets, R. G. Gordon, and D. F. Argus, *Geologically current plate motions*, Geophysical Journal International, 181 (2010), pp. 1–80.
[3] E. K. Donald et al., *The art of computer programming*, Sorting and searching, 3 (1999), p. 4.
[4] J. Durbin and S. J. Koopman, *Time series analysis by state space methods*, vol. 38, OUP Oxford, 2012.
[5] M. Gu, X. Fang, and Y. Lin, *FastGaSP: Fast and Exact Computation of Gaussian Stochastic Process*, 2025, https://CRAN.R-project.org/package=FastGaSP. R package version 0.6.1.
[6] R. E. Kalman, *A new approach to linear filtering and prediction problems*, Journal of basic Engineering, 82 (1960), pp. 35–45.
[7] R. E. Kalman and R. S. Bucy, *New results in linear filtering and prediction theory*, Journal of basic engineering, 83 (1961), pp. 95–108.
[8] A. Meucci, *Review of statistical arbitrage, cointegration, and multivariate Ornstein-Uhlenbeck*, Cointegration, and Multivariate Ornstein-Uhlenbeck (May 14, 2009), (2009).
[9] G. Petris, S. Petrone, and P. Campagnoli, *Dynamic linear models*, Springer, 2009.
[10] H. E. Rauch, F. Tung, and C. T. Striebel, *Maximum likelihood estimates of linear dynamic systems*, AIAA journal, 3 (1965), pp. 1445–1450.

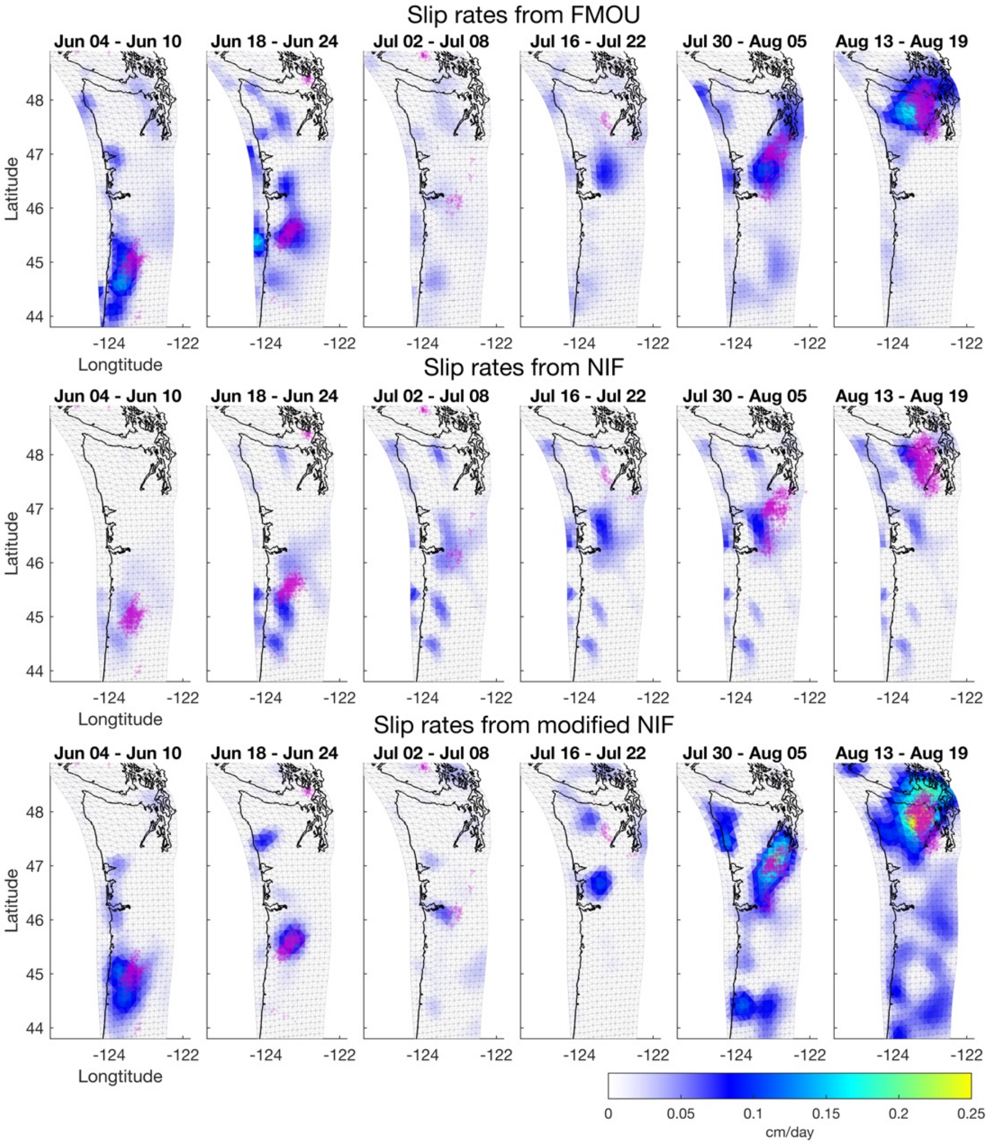


**Figure SM4.** *The seven-day averages of slip rates over the observed dates. Slip rates estimated by the FMOU, NIF and modified NIF are plotted in upper row, middle row and bottom row, respectively, for the Cascadia displacement data in 2011. The tremor epicenters are plotted as magenta dots.*


[11] P. Segall and M. Matthews, *Time dependent inversion of geodetic data*, Journal of Geophysical Research: Solid Earth, 102 (1997), pp. 22391–22409.

[12] J. H. Tu, C. W. Rowley, D. M. Luchtenburg, S. L. Brunton, and J. N. Kutz, *On dynamic mode decomposition: Theory and applications*, Journal of Computational Dynamics, 1 (2014), pp. 391–421.

[13] M. West and P. J. Harrison, *Bayesian Forecasting & Dynamic Models*, Springer Verlag, 2nd ed., 1997, http://www.stat.duke.edu/~mw/book.html.

[14] H. Wolkowicz, *A note on lack of strong duality for quadratic problems with orthogonal constraints*, European Journal of Operational Research, 143 (2002), pp. 356–364.
